# Supplementary material for: Person-in-Context Synthesiswith Compositional Structural Space
Source: arXiv:2008.12679 source file (2020-08-28)
Supplement: Supplementary file 1 [file supplementary.tex]

\begin{figure*}[b]
\begin{center}
   \includegraphics[width=0.91\linewidth]{supp_images/composed_im_0.png}
\end{center}
\caption{More COCO-Stuff Results for Comparision}
\end{figure*}

\begin{figure*}[b]
\begin{center}
   \includegraphics[width=0.91\linewidth]{supp_images/composed_im_1.png}
\end{center}
\caption{More COCO-Stuff Results for Comparision}
\end{figure*}
\begin{figure*}[b]
\begin{center}
   \includegraphics[width=0.91\linewidth]{supp_images/composed_im_2.png}
\end{center}
\caption{More COCO-Stuff Results for Comparision}
\end{figure*}
\begin{figure*}[b]
\begin{center}
   \includegraphics[width=0.91\linewidth]{supp_images/composed_im_1.png}
\end{center}
\caption{More COCO-Stuff Results for Comparision}
\end{figure*}
\begin{figure*}[b]
\begin{center}
   \includegraphics[width=0.91\linewidth]{supp_images/composed_im_4.png}
\end{center}
\caption{More COCO-Stuff Results for Comparision}
\end{figure*}
\begin{figure*}[b]
\begin{center}
   \includegraphics[width=0.91\linewidth]{supp_images/composed_im_5.png}
\end{center}
\caption{More COCO-Stuff Results for Comparision}
\end{figure*}
\begin{figure*}[b]
\begin{center}
   \includegraphics[width=0.91\linewidth]{supp_images/composed_im_6.png}
\end{center}
\caption{More COCO-Stuff Results for Comparision}
\end{figure*}
\begin{figure*}[b]
\begin{center}
   \includegraphics[width=0.91\linewidth]{supp_images/composed_im_7.png}
\end{center}
\caption{More COCO-Stuff Results for Comparision}
\end{figure*}
\begin{figure*}[b]
\begin{center}
   \includegraphics[width=0.91\linewidth]{supp_images/composed_im_8.png}
\end{center}
\caption{More COCO-Stuff Results for Comparision}
\end{figure*}
\begin{figure*}[b]
\begin{center}
   \includegraphics[width=0.91\linewidth]{supp_images/composed_im_9.png}
\end{center}
\caption{More COCO-Stuff Results for Comparision}
\end{figure*}
\begin{figure*}[b]
\begin{center}
   \includegraphics[width=0.91\linewidth]{supp_images/composed_im_10.png}
\end{center}
\caption{More COCO-Stuff Results for Comparision}
\end{figure*}
